# Supplementary material for: Locating Sycophancy Across Training Stages in Open Language Models
Source: arXiv:2610.37788 source file (2026-10-27)
Supplement: Supplementary file 1 [file appendix_main.tex]

\documentclass{article}          % whatever main.tex uses
\input{preamble}                 % same packages, macros, \cell, \appref, pgfplots setup
\usepackage{xr}
\externaldocument{main}          % lets \Cref{sec:multiturn}, \Cref{fig:stages} etc. resolve from main.aux
\begin{document}
\appendix
\input{appendix/appendix}

% \bibliography{iclr2027_conference}

% \bibliographystyle{iclr2027_conference}

\end{document}
